# Supplementary material for: Semiclassical Limit of Measurement-Induced Transition in Many-Body Chaos in Integrable and Nonintegrable Oscillator Chains
Source: arXiv:2210.03760 source file (2024-01-20)

UC 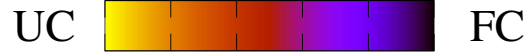 FC

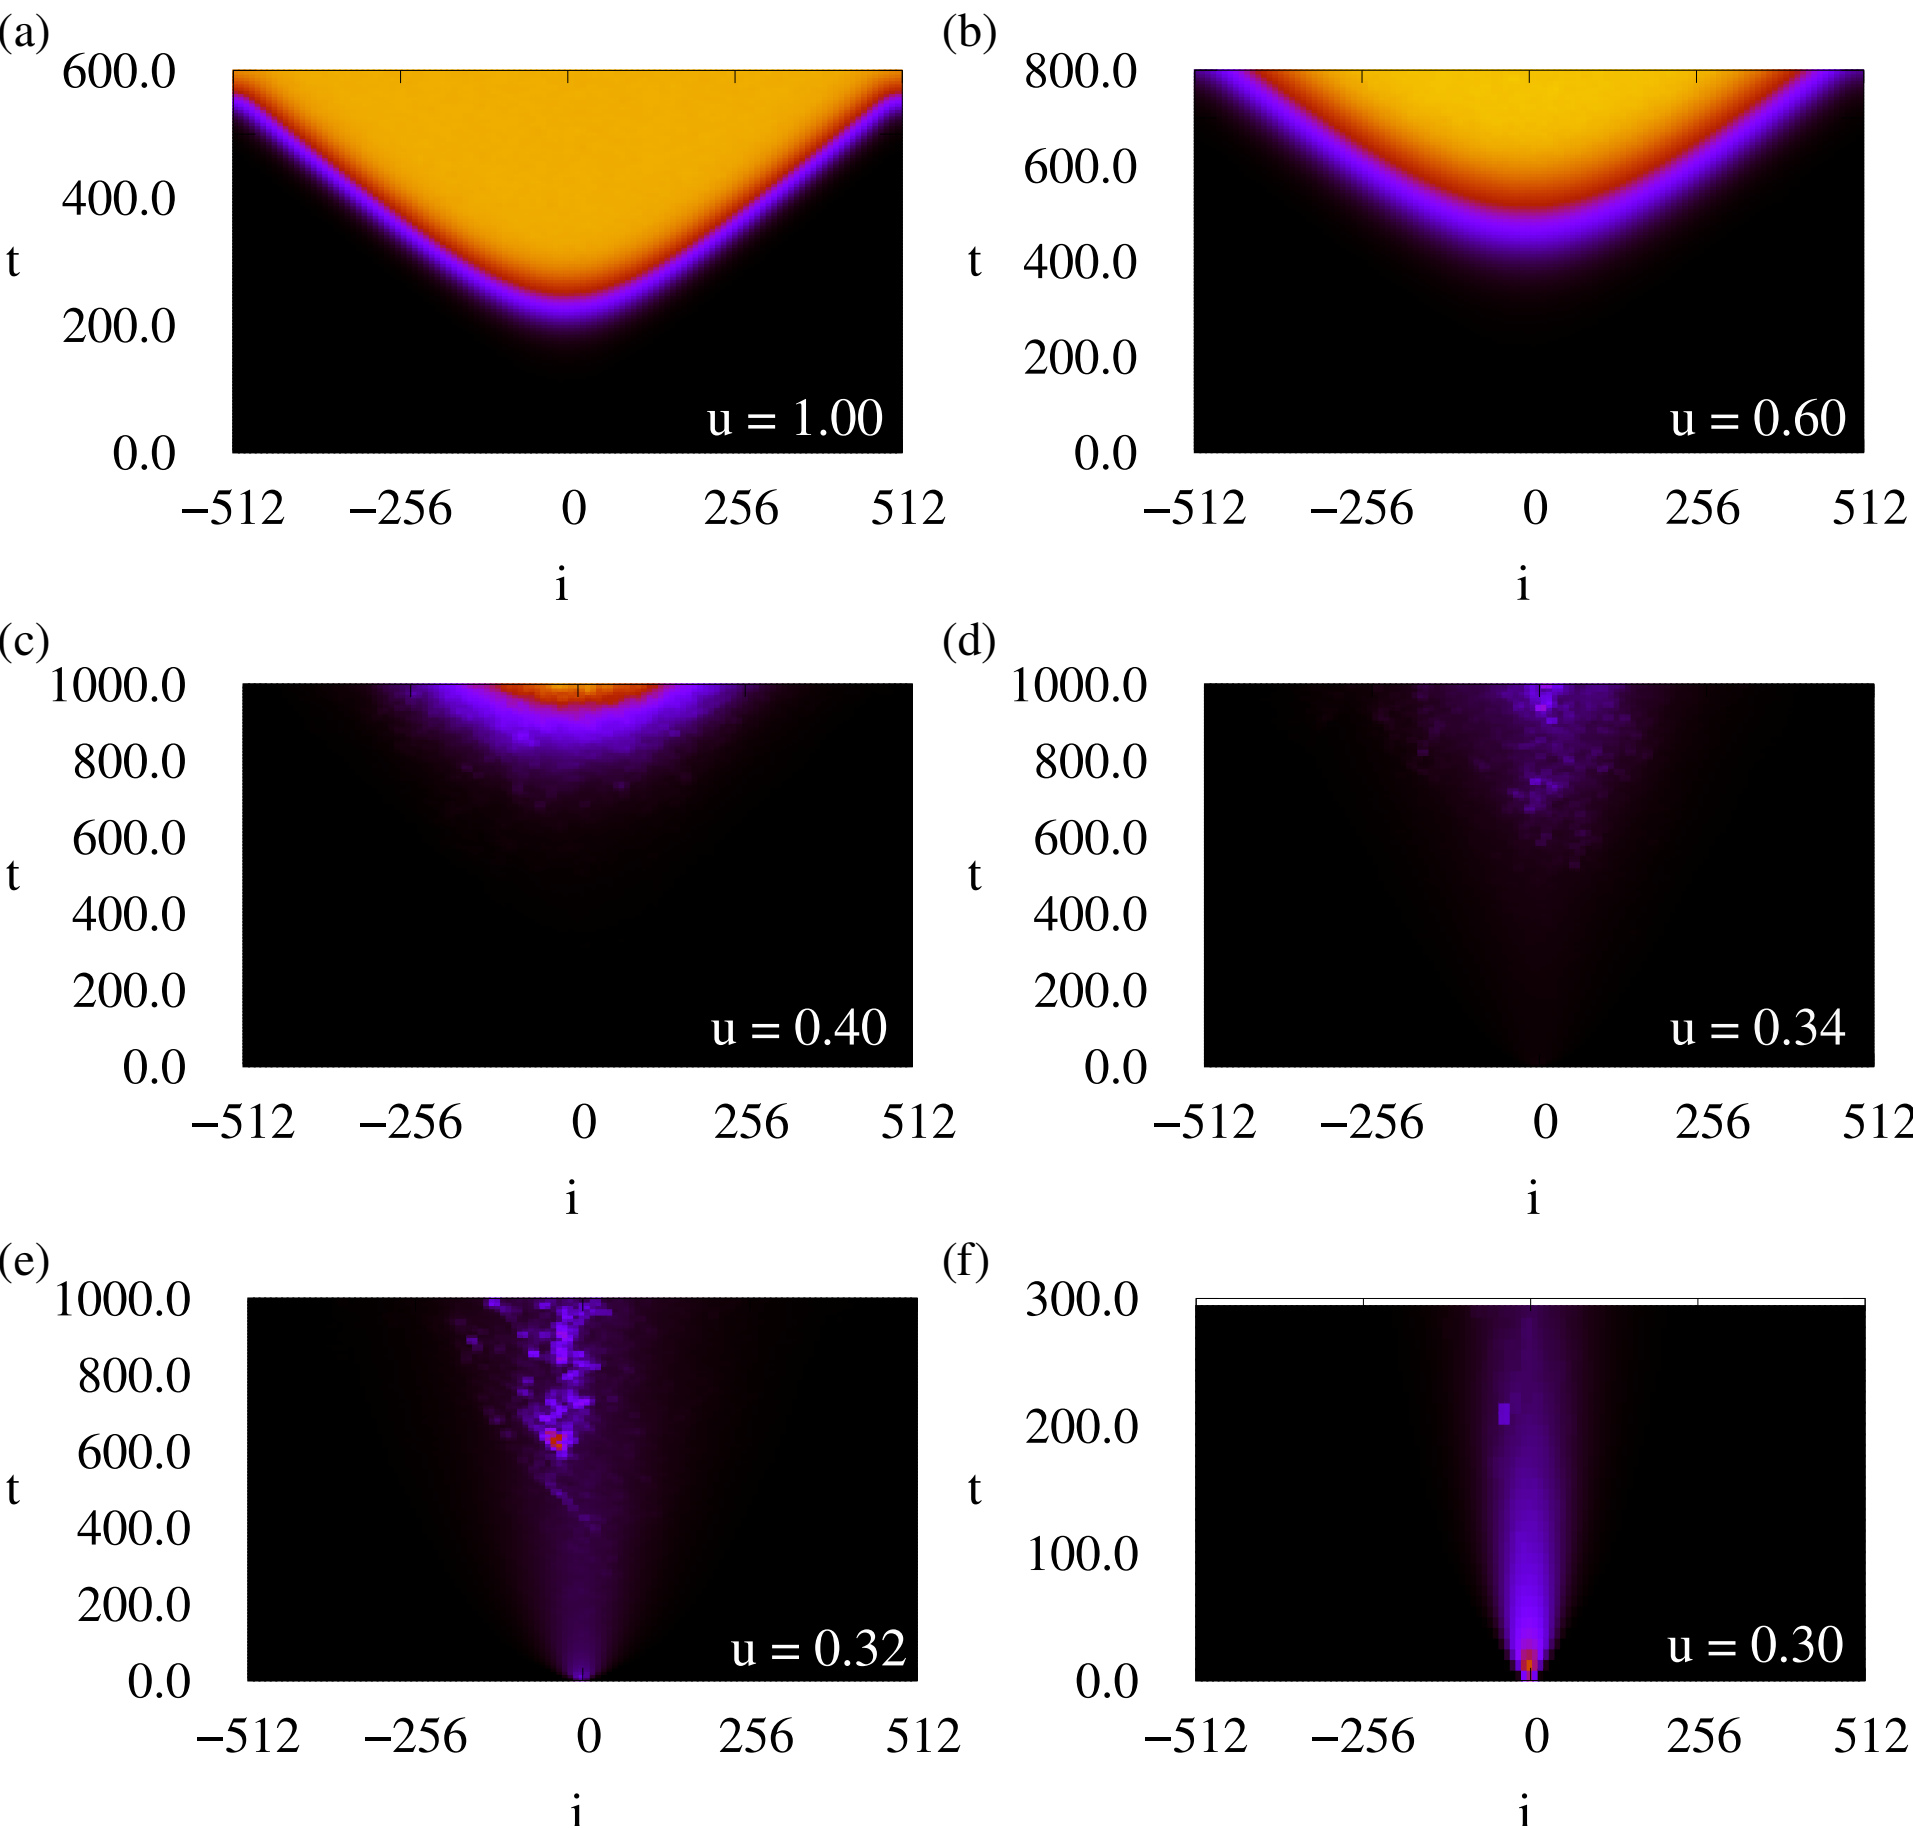

Supplement: Supplementary file 1 [file SM_LC_Transition.pdf]
